# Supplementary material for: Tracking and distinguishing slime mold solutions to traveling salesperson problems through synchronized amplification in the non-equilibrium steady state
Source: arXiv:2504.03492 source file (2026-09-22)
Supplement: Supplementary file 1 [file Supplementary_Material.pdf]

# Supplementary Material:

## Tracking and Distinguishing Slime Mold Solutions to the Traveling Salesman Problem through Synchronized Amplification in the Non-Equilibrium Steady State

Suyash Bajpai†, Masashi Aono‡, and Philip Kurian*,†

‡Amoeba Energy Co., Ltd., 2-15-1 Konan, Minato, Tokyo, Japan 108-6022

†Quantum Biology Laboratory, Howard University, Washington DC, 20060 USA

*E-mail: pkurian@howard.edu

# S1 Smoothening of $X_{Vk}$ and the Savitzky-Golay filter

We employ the Savitzky-Golay filter to smooth the $X_{Vk}$ signal and suppress noisy frequency components. When an appropriate window size is chosen, the slower, large-amplitude oscillations in the NESS for solution lanes become more discernible. The Savitzky-Golay-filtered $X_{Vk}$ plot now more clearly reveals the larger-scale frequency trends in the $X_{Vk}$ values of the solution lanes. Figure S1 shows a representative Savitzky-Golay plot for one of the solution lanes in the NESS. Notably, this filter has been widely used in electroencephalogram (EEG) signal processing, where preserving the original shape and amplitude of waveform features while reducing high-frequency noise is essential. Interestingly, EEG signals from the human brain closely resemble the cytosolic oscillations observed in this aneural organism [1] (Fig S1).

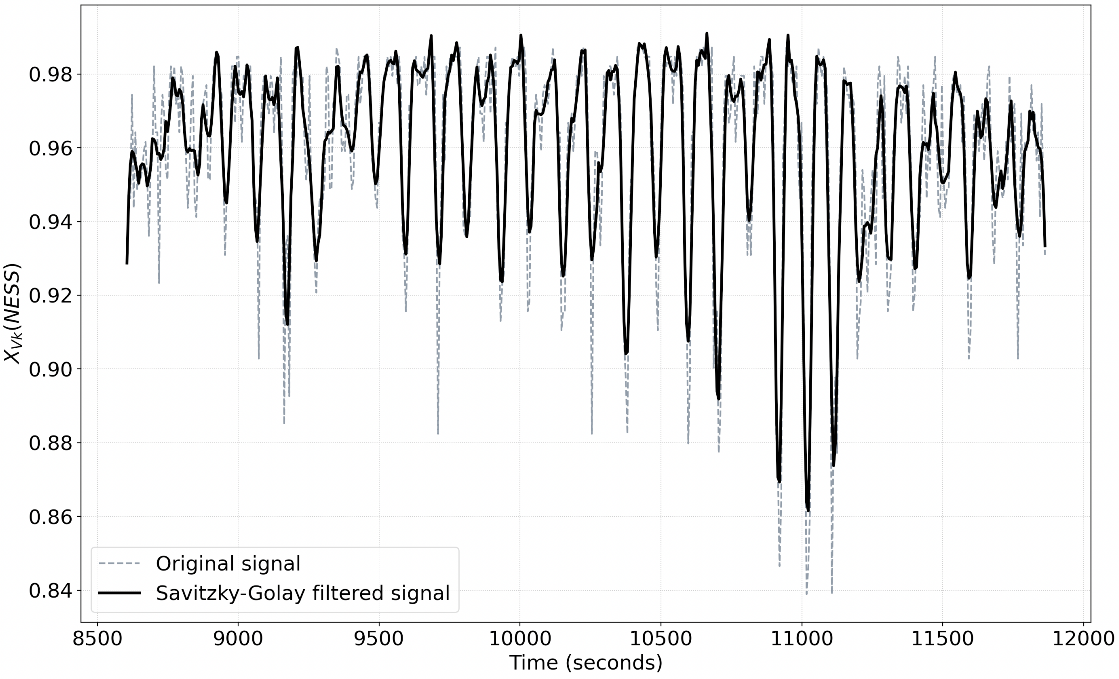


Figure S1: **Slower, large-amplitude oscillations become more evident for the solution lanes in the NESS region when processed using the Savitzky-Golay filter.** The figure illustrates the effect of smoothening on the $X_{Vk}$ signal of a solution lane using the Savitzky-Golay filter.

# S2 Power spectral density for various tour lengths

In addition to the power spectral density (PSD) plots shown for the solution with tour length 128 in Fig. 4 of the main text, we also analyzed the PSD plots for solutions with tour lengths 117, 122, 145, and 165 across the pre-illumination, optical feedback, and NESS regions. These solutions are considered "typical" as they follow the common $S(t)$ trend. For tour lengths 117, 122, and 145, the PSD plots (Fig. S2, a-i) consistently show a similar

frequency shift to that observed for tour length 128 (Fig. 4 in the main text): from a most prominent frequency of ∼0.02 Hz in the pre-illumination region to ∼0.01 Hz in the optical feedback and NESS regions. These plots also exhibit a clear amplification of the low-frequency signal in the solution lanes during the NESS phase. Though not the most prominent, the comparable faster component at ∼0.08 Hz is present across regions and tour lengths.

In contrast, the solution with tour length 165 exhibits markedly different behaviors (Fig. S2, j-l). In the pre-illumination region, both the solution and non-solution lanes show a lower most prominent frequency of ∼0.01 Hz. However, in the optical feedback and NESS regions, these two lane groups diverge in their frequency responses—and deviate from the typical behaviors observed in the other trials with shorter tour lengths. Specifically, the most prominent frequency in the solution lanes shifts to a higher value of ∼0.02 Hz during the optical feedback and NESS regions, whereas the non-solution lanes retain their dominant frequency at ∼0.01 Hz throughout all regions. Additionally, we do not observe any amplification in the strength of the most prominent frequency in the solution lanes during the NESS region, as compared to the optical feedback region. These deviations are due to the presence of irregularities and darker budding regions in the central processing hub of the *Physarum* body, which significantly affect the synchronization dynamics, as noted in the main text. Although tour 165 exhibits a typical $S(t)$ trend—justifying its inclusion with higher-quality, more pristine solutions—its structural anomalies are significant. For completeness, we also include tour length 165 among the anomalous cases in Section S5 below due to the presence of these irregularities.

# S3 Comparison of experiment and amoeba-inspired TSP algorithms

In experiments by Aono et al. [2], *Physarum* solved the TSP for $4 \leq N \leq 8$. It was shown that *Physarum* successfully found feasible solutions in all cases. Additionally, despite the increase in problem size from $N = 4$ to $N = 8$, *Physarum* was able to find good-quality solutions in almost linear time. These results suggested that the plasmodium has the ability to search for a reasonably high-quality solution at a low exploration cost, scaling in computation time with a near-linear dependence on the problem size. In contrast, the best approximate classical algorithms (such as the Lin-Kernighan heuristic, simulated annealing, or genetic algorithm) exhibited only a quadratic dependence at best.

We plotted the computation times for 4 to 8 cities, comparing *Physarum* with the Lin-Kernighan heuristic directly. As shown in Fig. 3a, in the range $4 \leq N \leq 8$, the computation time for *Physarum* shows a good linear fit ($R^2 = 0.98$), while the Lin Kernighan algorithm's computation time is best described by a quadratic fit ($R^2 = 1$). This remarkable observation suggests the presence of a parallel processing mechanism promoting computational speedups within *Physarum*'s body.

AmoebaTSP [2] and Improved AmoebaTSP [3], are two computational algorithms that were designed to mimic the solution-searching dynamics in the *Physarum*-based TSP-solving experiments. The differences between the two models are as follows: In the original Amoe-

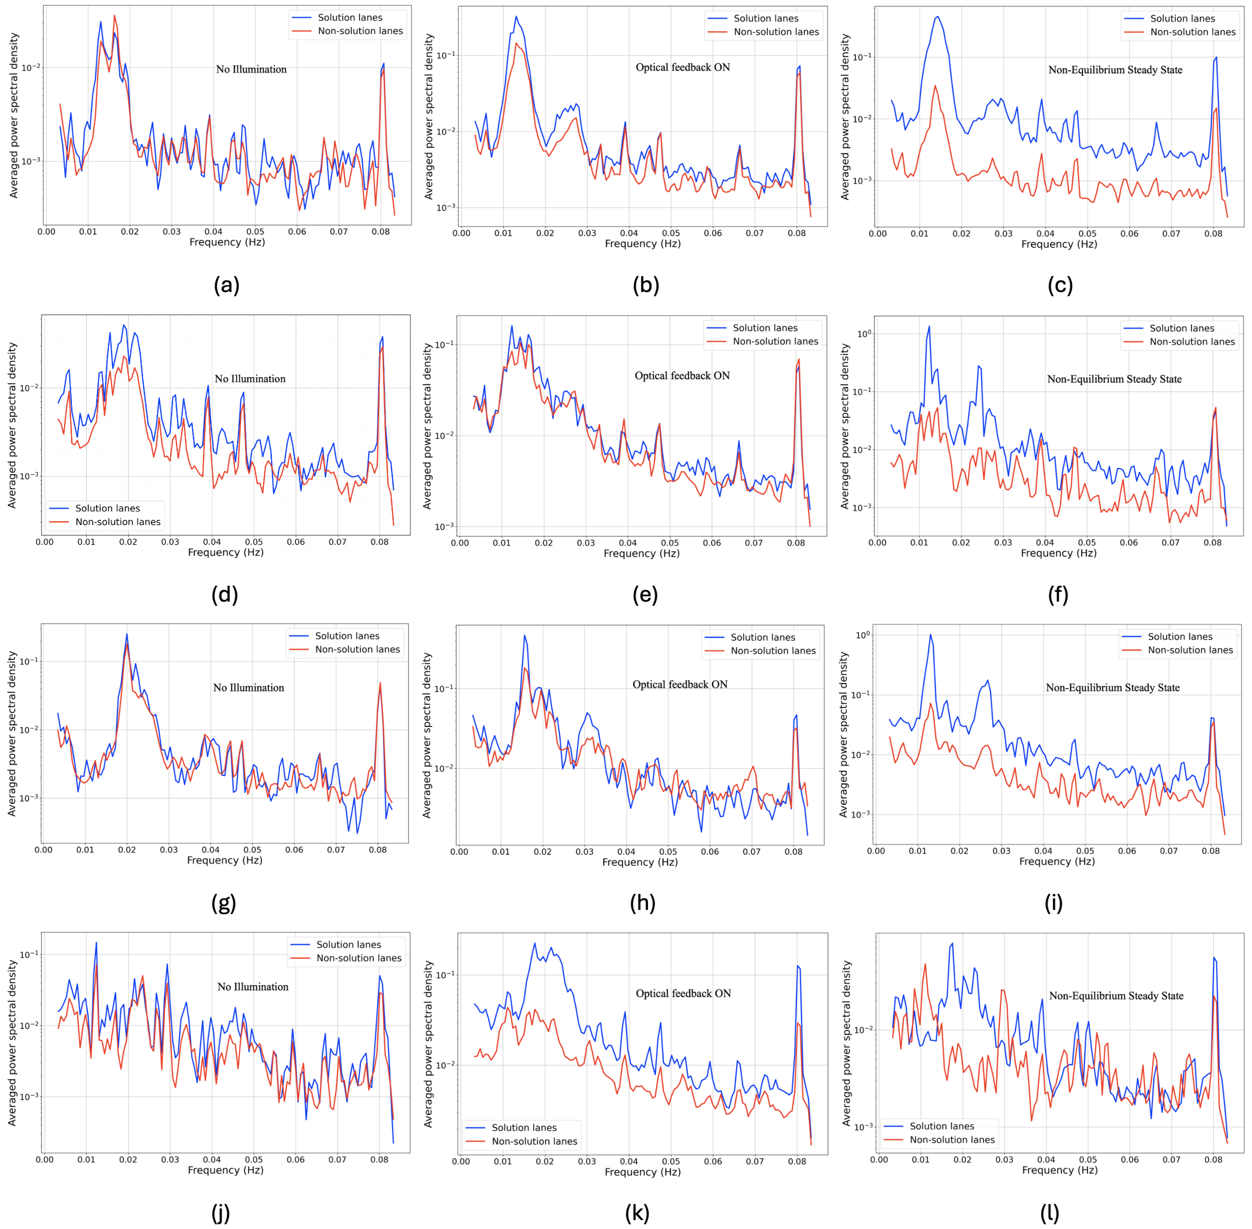


Figure S2: **The power spectral density (PSD) trends observed in the pre-illumination, optical feedback, and non-equilibrium steady-state (NESS) regions (as shown in Figure 4 of the main text) are consistently reproduced across different tour lengths.** Figures a–c represent the PSD plots for tour length 117 across the three regions. Similarly, Figures d–f show the PSD plots for tour length 122, Figures g–i present the PSD plots for tour length 145, while Figures j–l present the PSD plots for tour length 165 each analyzed in the pre-illumination, optical feedback, and NESS regions, respectively.

baTSP code, noise is added to the argument of the sigmoid function (Eq. 4 in the main text), whereas in the Improved AmoebaTSP model, it is applied directly to the $X_{Vk}$ updates. Additionally, the noise profile differs between the two models: the original AmoebaTSP uses

a uniform random noise, while the Improved AmoebaTSP employs a Gaussian random noise. Another key modification is in the outflux function $O_{Vk}$ which depends on $X_{Vk}$ in the original model but is independent of $X_{Vk}$ in the improved version. Furthermore, the improved AmoebaTSP model modifies the influx equation by using the problem size instead of the number of illuminated lanes, which was used in the original model.

These modifications significantly reduce the number of iterations (Fig. 3b, inset) and computation time (Fig. 3c, inset) in the Improved AmoebaTSP compared to the original AmoebaTSP. However, for $N = 10$ to $N = 30$, this reduction comes at the cost of a decrease in solution quality, compared to the original AmoebaTSP model (Fig. 3d).

Figures 3b and 3c compare the iteration and computation time scalings of these algorithms with the Lin-Kernighan-Helsgaun (LKH) heuristic. The LKH iteration data is sourced from Ref. [4] for non-Euclidean instances, while the Improved AmoebaTSP algorithm is evaluated across 1,000 trials for problem sizes ranging from $N = 10$ to $N = 100$ on another set of non-Euclidean instances. Our analysis reveals that, within the range of $N = 10$ to $N = 100$, the Improved AmoebaTSP algorithm exhibits a scaling trend similar to the LKH heuristic. However, it demonstrates slightly better scaling in both iteration count ($\sqrt{N}$ for Improved AmoebaTSP compared to $N^{0.65}$ for LKH) and computation time. While the overall scaling behavior of Improved AmoebaTSP remains close to LKH, it exhibits a slight computational scaling advantage, even though the LKH is three orders of magnitude faster (more time-efficient) at a given problem size. Figure 4 shows the normalized distance maps for representative 29-city non-Euclidean TSP instances used in the LKH heuristic (bays29 from the TSPLIB dataset [5]) and in our calculations. For computation-time comparisons, we utilized the empirical fit from the LKH report [6]. The observed similarity in scaling trends is particularly intriguing, motivating a deeper investigation into the problem-solving capabilities of *Physarum*-based computing and suggesting potential opportunities to hybridize LKH and amoeba-inspired algorithms for even more effective TSP search.

The difficulty of a TSP instance can be assessed by its distance matrix. Both our instance and the TSPLIB bays29 instance have distances normalized between 0 and 1, but their structures differ (Figure S4). bays29 (Figure S4a) shows clear low-distance clusters (bluer regions), suggesting tight groupings of nearby cities and a more structured pattern. Our instance lacks such clustering, with more distances concentrated between 0.5 and 1 (redder regions) — indicating that while city-to-city distances are large, they are still sufficiently distinct to obviate repetitive structure (Fig. S4b). This is reflected in the determinant of our distance matrix ($2.9 \times 10^{-7}$), which is much larger than that of bays29 ($8.3 \times 10^{-25}$), implying greater structural independence among distances and potentially higher difficulty of the problem. Although the determinant is not the only figure of merit used to assess the complexity of an instance, the overall structure plays a key role: instances with more spatial or distance-based structure are generally easier to solve than unstructured problems, as discussed in the main text.

Addressing noise is crucial in *Physarum*-inspired algorithms to ensure effective convergence to a solution. In the original AmoebaTSP algorithm, the system fails to converge when no noise is introduced, resulting in no solution. This is consistent with the findings in Refs. [7, 8], which suggest that adaptation does not occur in the absence of noise. In experiments, thermal and optical noise naturally present in *Physarum* aid adaptation to the applied illumination and help the organism discriminate its growth between lane groups to solve a TSP

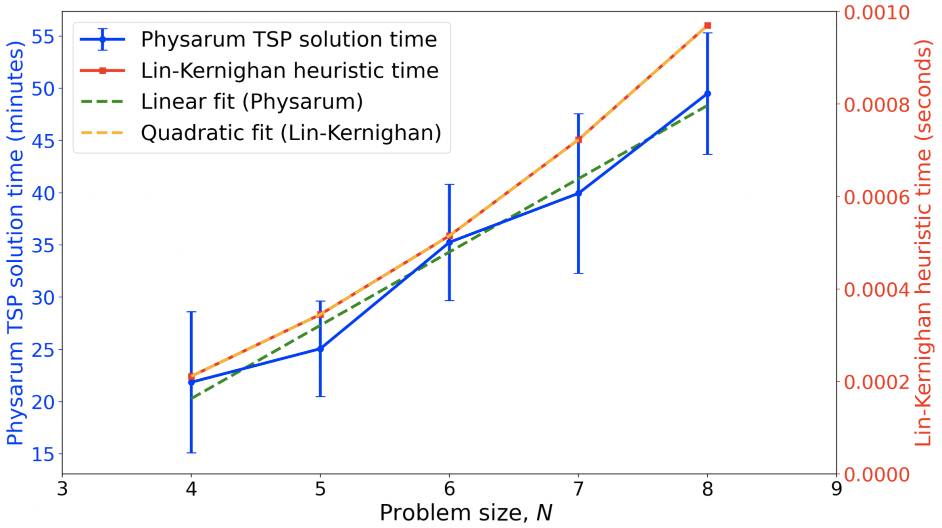
Physarum TSP solution time
Lin-Kernighan heuristic time
Linear fit (Physarum)
Quadratic fit (Lin-Kernighan)
Physarum TSP solution time (minutes)
Lin-Kernighan heuristic time (seconds)
Problem size, N

**(a)**

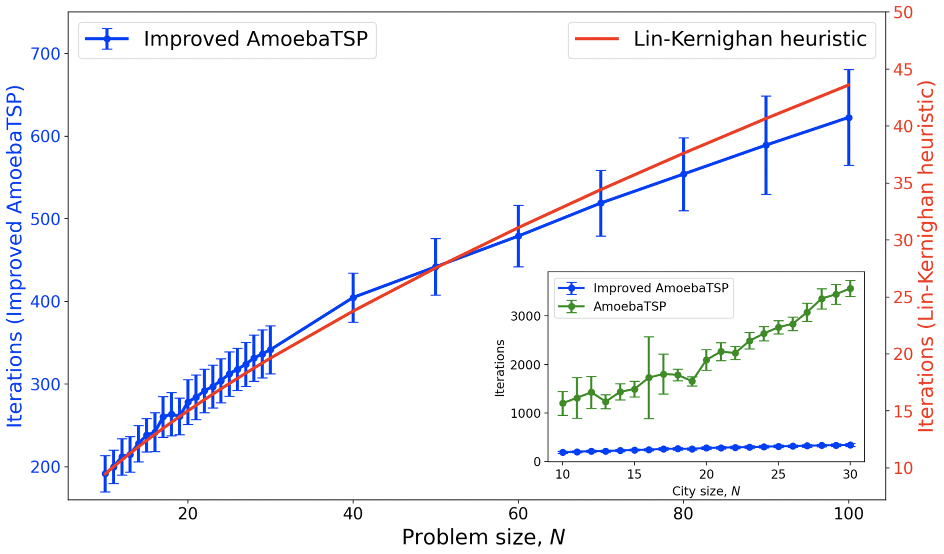
Improved AmoebaTSP
Lin-Kernighan heuristic
Iterations (Improved AmoebaTSP)
Iterations (Lin-Kernighan heuristic)
Problem size, N
Improved AmoebaTSP
AmoebaTSP
Iterations
City size, N

**(b)**

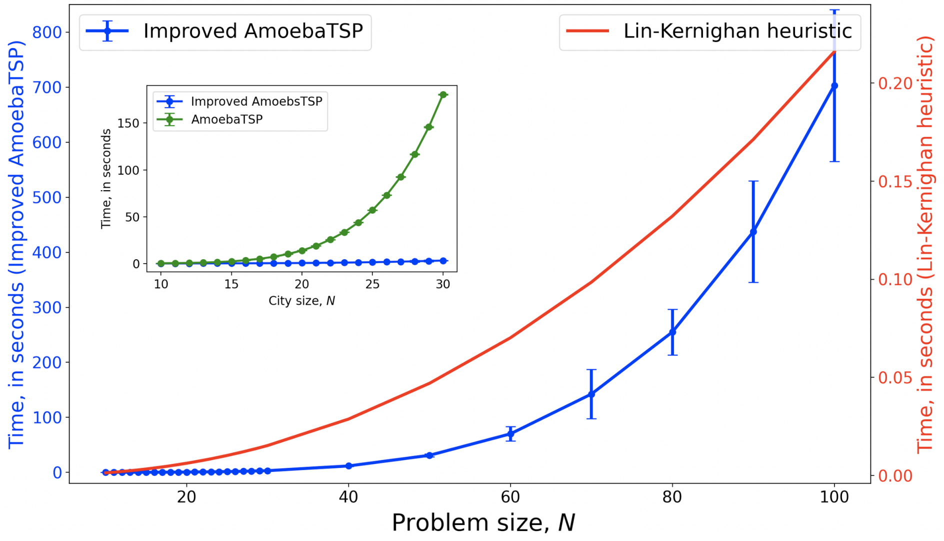
Improved AmoebaTSP
Lin-Kernighan heuristic
Time, in seconds (Improved AmoebaTSP)
Time, in seconds (Lin-Kernighan heuristic)
Problem size, N
Improved AmoebsTSP
AmoebaTSP
Time, in seconds
City size, N

**(c)**

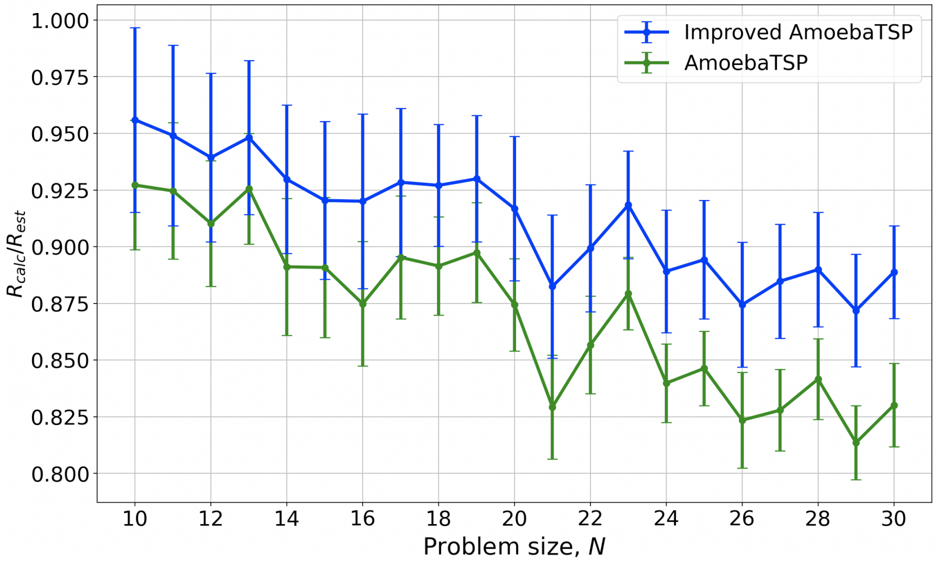


**(d)**

Figure S3: ***Physarum's* TSP computation time scales linearly with problem size for small instances ($N \leq 8$), whereas one of the most widely used classical TSP algorithms exhibits superquadratic scaling, suggesting potential information processing speedups within the amoeba.** (a) The panel shows the comparison of scalings of the *Physarum* TSP solution time (blue) and the Lin-Kernighan heuristic (LKH) algorithm time (red) with the problem size $N$. *Physarum* exhibits a linear scaling of solution time with $N$, as indicated by the dashed green linear fit. In contrast, the LKH implementation shows superquadratic ( $\sim N^{2.2}$) scaling, represented well for low $N$ by the dashed yellow quadratic fit. Comparison between (b) iterations as well as (c) computational time scalings of the LKH, and *Physarum*-inspired AmoebaTSP and Improved AmoebaTSP algorithms for a much larger range of TSP problem sizes ($10 \leq N \leq 100$). (d) Comparison of the ratio of calculated vs. mean tour lengths for AmoebaTSP and Improved AmoebaTSP for $10 \leq N \leq 30$. A lower ratio indicates a higher solution quality.

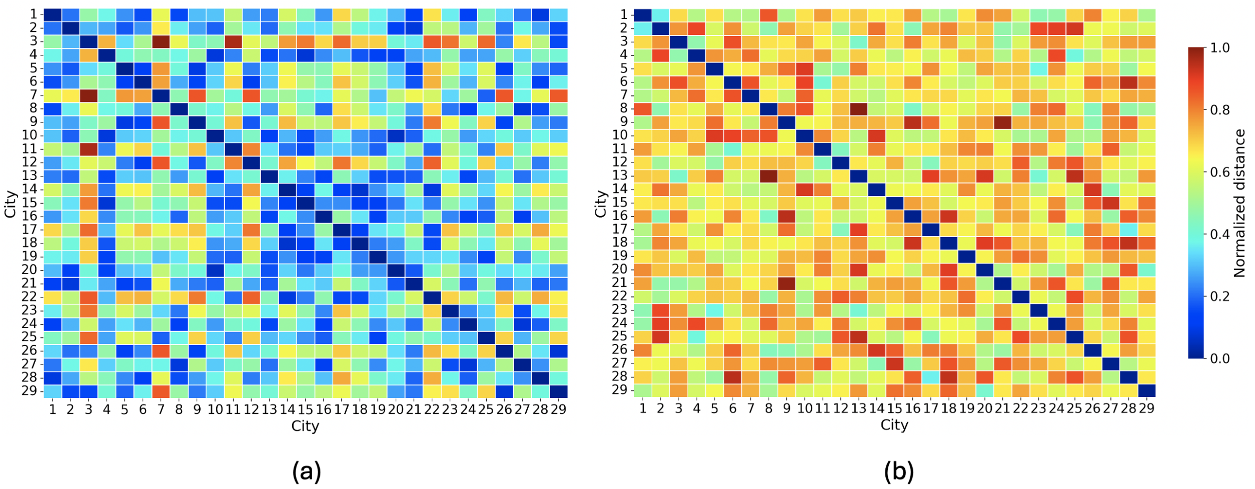


Figure S4: Color-coded distance maps for two distinct 29-city, non-Euclidean TSP instances, with distances normalized between 0 and 1. (a) bays29 instance from the TSPLIB dataset [5], and (b) the corresponding instance used in our study. Both maps use the same heatmap color bar, shown alongside panel (b).

instance. In the original AmoebaTSP algorithm, when uniform random noise is added to the activation function, the system finds shorter paths but at the cost of requiring a higher number of iterations. In contrast, when noise is directly added to the $X_{Vk}$ update steps or when a Gaussian noise distribution replaces uniform noise, the number of iterations decreases, leading to faster convergence, albeit with longer tour lengths. Additional modifications to the Improved AmoebaTSP model—such as making the outflux update term independent of $X_{Vk}$—further reduce iteration counts but similarly result in longer tour lengths. Though these modifications reduce the scaling of iteration count with problem size to $\sqrt{N}$ in the Improved AmoebaTSP algorithm, they come at the expense of solution quality.

As stated above, these observations are consistent with Refs. [7, 8], which highlight that adaptation is optimal only at a well-tuned noise level. This emphasizes a fundamental trade-off in noise-driven optimization: too little noise prevents convergence, while excessive noise disrupts solution quality. The effective bifurcation in synchronization indices between solution and non-solution lanes arises from *Physarum*'s driven, dissipative dynamics assisted by environmental noise. If the noise level exceeds an optimal threshold, this trend deviates from the typical $S(t)$ behavior. For instance, additional noise from anomalous growths in the circular processing hub of the chip manifests as irregularities in the $S(t)$ time series (Figs. S6b,d). Further experiments with *Physarum* are needed to determine the optimal noise level, which could be leveraged to obtain higher-quality solutions more efficiently.

In the experiment [2], Gaussian white noise with a flat power spectral density, $\xi_{Vk}(t) \in [-d, d]$, where $d$ denotes the noise level, was added to $X_{Vk}(t)$. Consequently, in the optical feedback control, the input was replaced with a noise-perturbed argument, $X_{Vk}(t) + \xi_{Vk}(t)$. Since the noise is generated randomly and without temporal or spatial correlation, it disrupts the coordinated dynamics between branches, significantly affecting the success rate of the TSP solution.

This observation motivates the exploration of alternative activation functions (Table

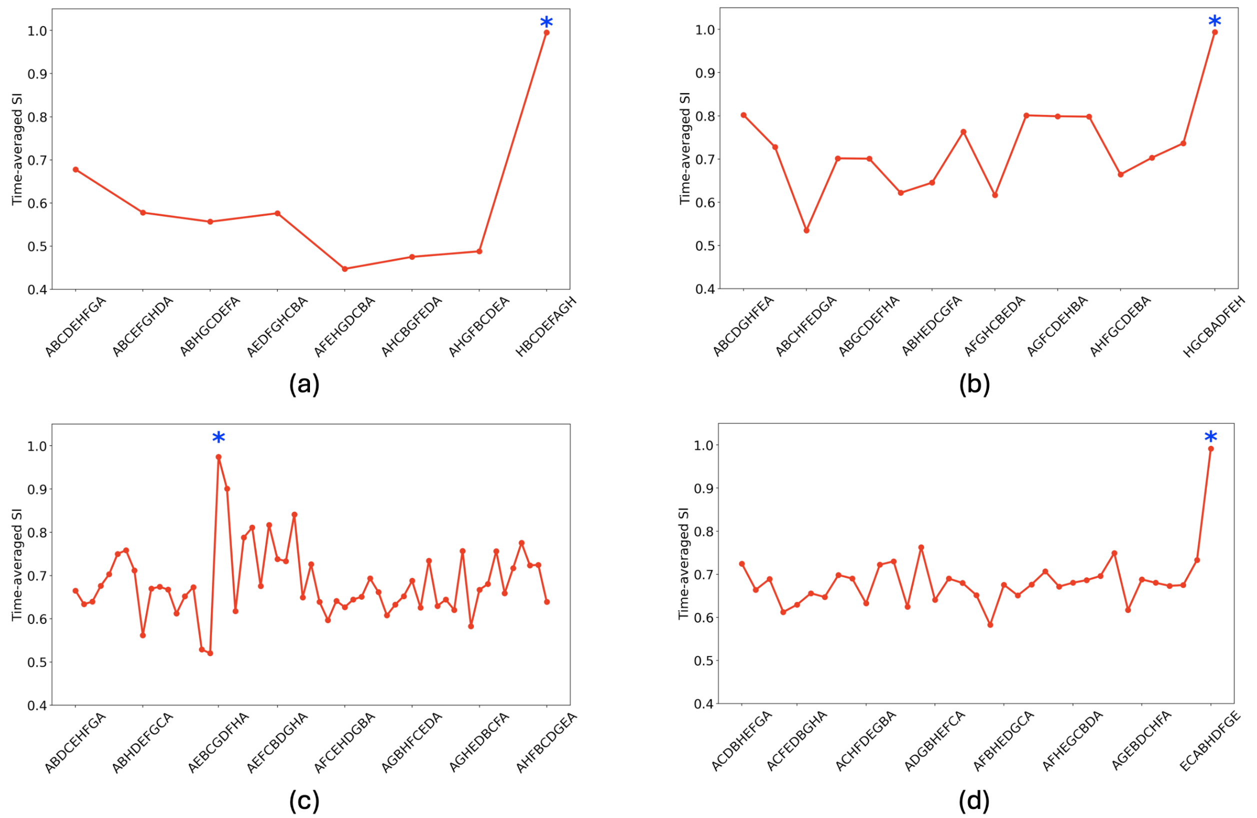


Figure S5: Time-averaged synchronization indices ($S'$) in the NESS, plotted for all distinct tours corresponding to a particular tour length, with the peak indicating the $S'$ value of the solution chosen by *Physarum* (marked by the asterisk). We list tours in lexicographic (dictionary) order by city label, from the first position to the last. Specifically, we first compare which city occupies the first position; among all tours sharing the same first city, we then compare the second city, and so on, until we have a complete ordering of all tours. (a) Tour length = 117 (b)Tour length = 122 (c) Tour length = 145 (d) Tour length = 165.

S1), which may enhance the system's robustness against such uncorrelated noise and help preserve performance. Moreover, if an optimal noise distribution can be identified (as discussed earlier), a modified activation function can potentially improve the overall efficiency of *Physarum* in solving the TSP. A tailored activation function based on Gaussian white noise in the Langevin equations would be ideal in this case, as the Langevin equations can describe stochastic behaviors such as those exhibited in *Physarum*.

# S4 Comparison of $S'$ values in *Physarum*-selected tours vs. other distinct tours

Similar to Fig. 6b in the main text, we compared the time-averaged synchronization indices ($S'$) of the *Physarum*-selected solutions with those of other distinct tours of the same tour length, for various tour lengths. As expected, the $S'$ values for the *Physarum*-selected tours

are the highest (each marked with an asterisk), as shown in Fig. S5.

# S5 Anomalous *Physarum* solutions

## S5.1 Time-dependent sychronization behavior of anomalous solutions

When *Physarum* solves the TSP, it can provide high-quality solutions in linear time for problem sizes ranging from $N = 4$ to $N = 8$. In these solutions, the solution (non-solution) lanes are highly synchronized (desynchronized), following the trends presented in Figures 5–8 of the main text.

However, in some cases, the *Physarum* body exhibits anomalies, particularly in the central circular disk of the *Physarum* chip. These anomalies arise when the central part of the *Physarum* body is damaged or shows irregular growth patterns. Certain darker budding regions emerge in this circular area, disrupting the oscillator dynamics of *Physarum* and consequently affecting its synchronization behavior.

This disturbance alters the synchronization dynamics between the solution and non-solution lanes, leading to deviations from the expected synchronization index ($S(t)$) trends observed in Fig. 5a of the main text. Panels S6a-d show solutions with tour lengths 123 and 162, where the presence of these darker budding regions significantly disrupts the oscillatory dynamics, resulting in large deviations from the typical $S(t)$ trend. In contrast, Figs. S6e-f show a solution with tour length 165, where such darker budding regions still affect the oscillatory behaviors, keeping the overall $S(t)$ trend intact (Fig. S6f) but with more pronounced fluctuations in the order parameter values. Owing to the preservation of the characteristic $S(t)$ trend, the solution with tour length 165 is grouped with the higher-quality, pristine tours, both here and in the main text. The PSD plots for the anomalous solutions with tour lengths 123 and 162 are provided in Section S5.2.

It is particularly interesting that, despite the presence of darker budding regions disrupting the central processing hub, *Physarum* was still able to find valid solutions to the eight-city TSP problem. This suggests that even when parts of its main body are disrupted, *Physarum* adapts to the disturbance by redistributing its internal resources, thereby altering its synchronization dynamics. These perturbed dynamics may deviate from the typical patterns observed in Fig. 5a of the main text, with the nature of the deviation depending on the extent of the disturbance. In some cases, we observe a clear reduction in the overall $S(t)$ trend (Fig. S6a-d), indicative of larger disruptions. In other cases, such as in Fig. S6e-f, the $S(t)$ trend appears similar to the typical behavior but with pronounced fluctuations, possibly reflecting milder disturbances. Further tests are needed to investigate *Physarum*'s adaptive mechanisms in response to such perturbations induced by the applied light field.

## S5.2 Power spectral density of anomalous solutions

Fig. S7 shows the PSD plots for the anomalous solutions with tour lengths 123 and 162, whose synchronization dynamics are significantly affected by disturbances in the central processing hub. As shown in panels S7a–f, while both tours exhibit prominent frequency

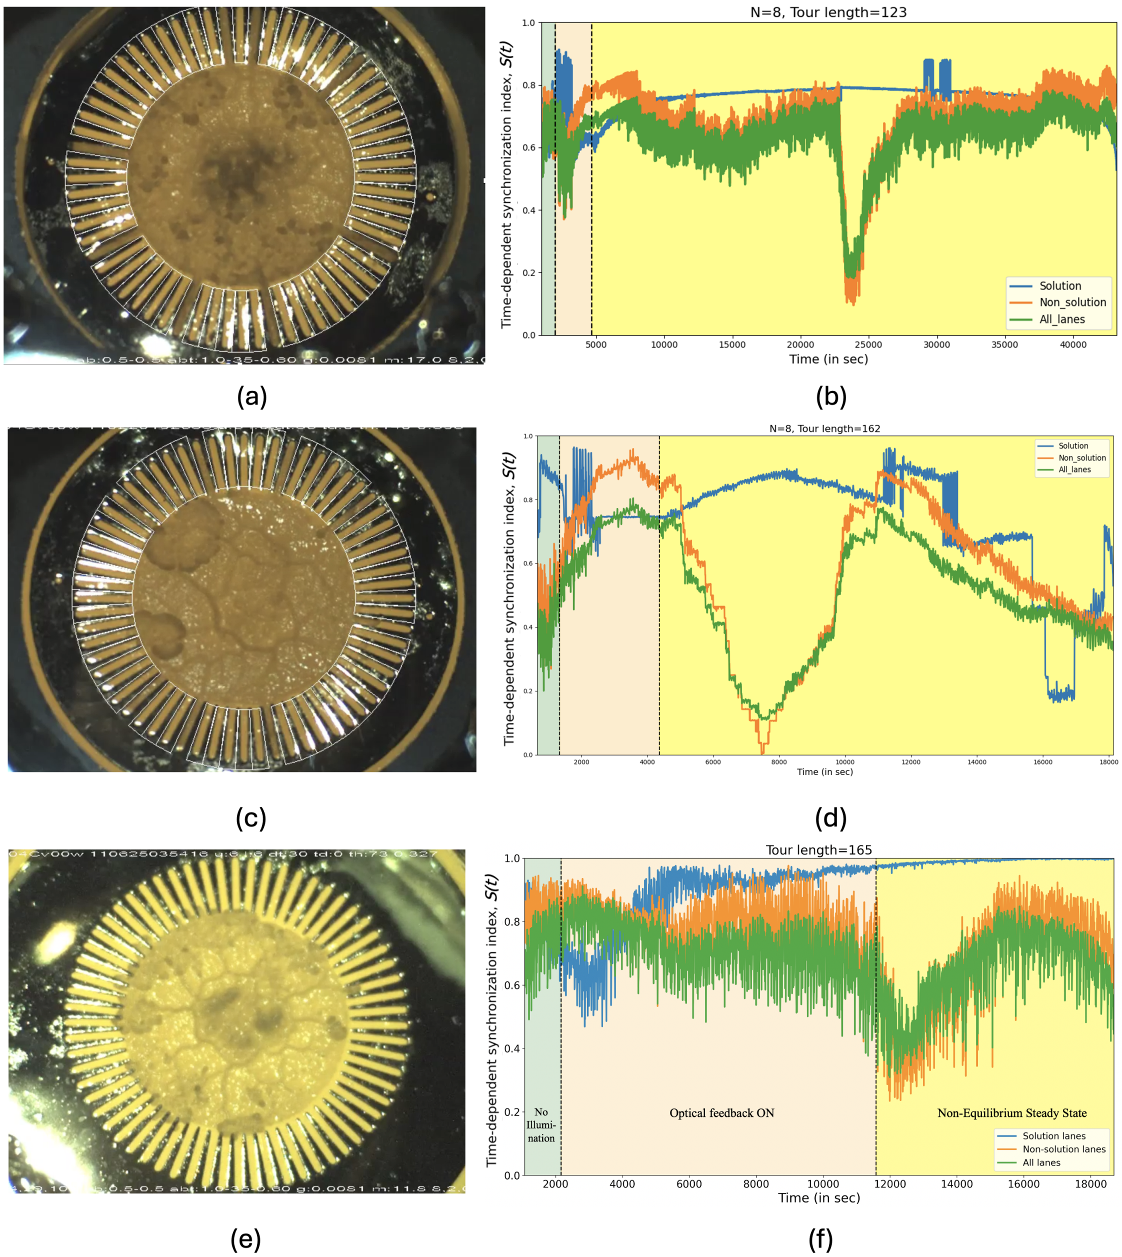


Figure S6: **Anomalous growth patterns in the central hub of the *Physarum* body disrupt synchronization dynamics, causing deviations in $S(t)$ values from the time-series trends observed in solutions with a more coherent central processing hub.** The figure shows (a) a snapshot of *Physarum* solving the TSP, displaying darker budding patterns in the central hub for a tour length of 123, (b) the $S(t)$ time series exhibiting anomalous deviations for the tour length of 123, (c) a snapshot of *Physarum* solving the TSP, displaying darker budding patterns in the central hub for a tour length of 162, (d) the $S(t)$ time series exhibiting anomalous deviations for the tour length of 162, (e) a snapshot of *Physarum* solving the TSP, displaying darker budding patterns in the central hub for a tour length of 165, and (f) the $S(t)$ time series exhibiting more significant fluctuations for the tour length of 165.

components in the $\sim 0.01$ Hz region—a feature observed in typical solutions—neither tour demonstrates amplification in the strength of the most prominent frequency signal for solution lanes in the NESS, compared to the optical feedback region. In fact, the opposite trend is observed: the strength of the most prominent frequency signal is suppressed from the optical feedback region to the NESS. This provides evidence that such disturbances impair the synchronization dynamics of *Physarum*, potentially deteriorating its efficiency in solving the problem, even though valid TSP solutions are arrived at in both cases (and a high-quality solution in the case of tour length 123). The average PSD analysis can be used to characterize a typical solution if it exhibits a shift from higher to lower frequencies from the pre-illumination to the optical feedback region, along with an amplification in the strength of the most prominent frequency component for solution lanes, as they evolve from the optical feedback to the NESS.

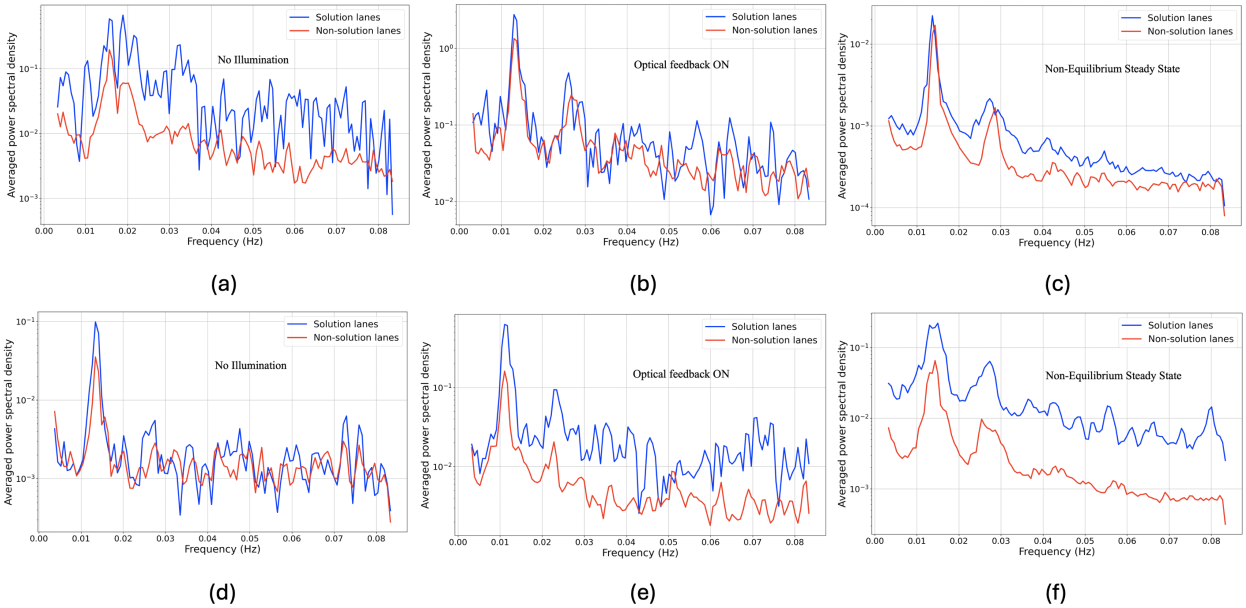


Figure S7: **The power spectral density (PSD) trends observed for anomalous *Physarum* solutions fail to exhibit amplification of the most prominent solution lane signal components in the non-equilibrium steady state (NESS), instead suppressing them.** Panels a–c represent the PSD plots for selected tour length 123 across pre-illumination, optical feedback, and NESS regions. Similarly, panels d–f show the PSD plots for selected tour length 162, analyzed for each of the same three regions, respectively.

# S6 Optical feedback control and activation functions for the modified Hopfield neural network

In earlier works, a sigmoid function was employed as the activation function in the optical feedback control. However, given the recent developments and applications in neural network implementations [9], a comparative analysis is warranted across several activation functions

(Table S1), including the rectified linear unit (ReLU) and its variants, the hyperbolic tangent (tanh), modified step functions, the exponential linear unit (ELU) and its variants, and others. We plan to investigate which of these activation functions most effectively optimizes the driven, dissipative dynamics of *Physarum* while solving the TSP under optical feedback control.

Table S1: Activation functions for neural network control

| **Activation Function** | **Mathematical Formulation** | **Description** |
|---|---|---|
| **Step** | $\Theta(x-a)=\begin{cases}0, & \text{if } x<a\\ 1, & \text{if } x\geq a\end{cases}$ | Simple threshold function; non-differentiable and rarely used in practice. |
| **Linear** | $f(x)=x$ | Identity mapping; lacks non-linearity, limiting expressive power. |
| **Sigmoid** | $f(x)=\frac{1}{1+e^{-\gamma(x-\theta)}}$ | Smooth, bounded function; suffers from vanishing gradients. |
| **Hyperbolic tangent** | $f(x)=\tanh(x)$ | Zero-centered alternative to sigmoid; still prone to gradient issues. |
| **Rectified Linear Unit (ReLU)** | $f(x)=\max(0,x)$ | Efficient and widely used; may lead to inactive neurons (dying ReLU). |
| **Leaky ReLU** | $f(x)=\max(\alpha x,x),\ 0<\alpha<1$ | Allows small gradient when $x<0$ to reduce dying ReLU effect. |
| **Parametric ReLU** | $f(x)=\max(\alpha x,x),\ \alpha$ learned | Learnable slope improves flexibility in learning. |
| **Exponential Linear Unit (ELU)** | $f(x)=\begin{cases}x, & x\geq 0\\ \alpha(e^x-1), & x<0\end{cases}$ | Pushes mean activation closer to zero; smoothens learning. |

| Activation Function | Mathematical Formulation | Description |
|---|---|---|
| **Swish** | $f(x) = \frac{x}{1+e^{-\gamma(x-\theta)}}$ | Non-monotonic, trainable function with empirical benefits. |
| **Scaled ELU** | $f(x) = \begin{cases} \lambda x, & x > 0 \\ \lambda\alpha(e^x - 1), & x \leq 0 \end{cases}$ | Self-normalizing; used in specific deep architectures. |
| **Softplus** | $f(x) = \ln(1 + e^x)$ | Smooth ReLU approximation; non-zero gradients everywhere. |
| **Softmax** | $f_i(x) = \frac{e^{x_i}}{\sum_j e^{x_j}}$ | Outputs a probability distribution over classes. |
| **Gaussian** | $f(x) = e^{-x^2}$ | Localized response; common in radial basis networks. |

# References


[1] Boussard, A. *et al.* Adaptive behaviour and learning in slime moulds: the role of oscillations. *Philosophical Transactions of the Royal Society B* **376**, 20190757 (2021).

[2] Zhu, L., Kim, S.-J., Hara, M. & Aono, M. Remarkable problem-solving ability of unicellular amoeboid organism and its mechanism. *Royal Society Open Science* **5**, 180396 (2018).

[3] Miyajima, Y. & Mochizuki, M. Proposed modified computational model for the amoeba-inspired combinatorial optimization machine. *Nonlinear Theory and Its Applications (NOLTA), IEICE* **15**, 824–837 (2024).

[4] Idzenga, A. *Experimental Analysis of the Lin-Kernighan heuristic*. B.S. thesis, University of Twente (2023).

[5] Reinelt, G. TSPLIB—A Traveling Salesman Problem Library. *ORSA Journal on Computing* **3**, 376–384 (1991).

[6] Helsgaun, K. An effective implementation of the Lin–Kernighan traveling salesman heuristic. *European journal of operational research* **126**, 106–130 (2000).

[7] Folz, F., Mehlhorn, K. & Morigi, G. Interplay of periodic dynamics and noise: Insights from a simple adaptive system. *Physical Review E* **104**, 054215 (2021).

[8] Folz, F., Mehlhorn, K. & Morigi, G. Noise-induced network topologies. *Physical Review Letters* **130**, 267401 (2023).

[9] Hopfield, J. J. Physics is a point of view. Nobel Prize lecture, Aula Magna, Stockholm (Dec 8, 2024) (2024). URL `https://www.nobelprize.org/prizes/physics/2024/hopfield/lecture/`. Nobel Prize in Physics 2024 laureate lecture.
